# Supplementary material for: Chiral phonons and phononic birefringence in ferromagnetic metal - bulk acoustic resonator hybrids
Source: arXiv:2303.08429 ancillary file (2023-03-15)
Supplement: Supplementary file 1 [file Supplementary_Material.pdf]

# Supplemental Material: Chiral phonons and phononic birefringence in ferromagnetic metal - bulk acoustic resonator hybrids

M. Müller,[1,2,*] J. Weber,[1,2] F. Engelhardt,[3,4,5] V. A. S. V. Bittencourt,[6] T. Luschmann,[1,2,7] M. Cherkasskii,[5] S.T.B. Goennenwein,[8] S. Viola Kusminskiy,[5,3] S. Geprägs,[1] R. Gross,[1,2,7] M. Althammer,[1,2,†] and H. Huebl[1,2,7,‡]

[1] *Walther-Meißner-Institut, Bayerische Akademie der Wissenschaften, 85748 Garching, Germany*
[2] *Technical University of Munich, TUM School of Natural Sciences, Physics Department, 85748 Garching, Germany*
[3] *Max Planck Institute for the Science of Light, 91058 Erlangen, Germany*
[4] *Department of Physics, University Erlangen-Nuremberg, 91058 Erlangen, Germany*
[5] *Institute for Theoretical Solid State Physics, RWTH Aachen University, 52074 Aachen, Germany*
[6] *ISIS (UMR 7006), Université de Strasbourg, 67000 Strasbourg, France*
[7] *Munich Center for Quantum Science and Technology (MCQST), 80799 Munich, Germany*
[8] *Department of Physics, University of Konstanz, 78457 Konstanz, Germany*
(Dated: March 15, 2023)

## I. Determination of the parameters describing the magnetization dynamics in CoFe

The parameters describing the magnetization dynamics are important to characterize the magnetic system. To determine these parameters, we have performed broadband ferromagnetic resonance (FMR) experiments. We fit the raw data as described in Ref. [1] and extract the FMR resonance frequency and linewidth in a frequency spacing in the GHz range, where the contributions from the elastic resonances average out. Fig. S1(a) and (b) show exemplary data for the resonance field $H_{\mathrm{res}}(f)$ and linewidth $\Delta H(f)$ of the $Al_2O_3$/CoFe sample at $T = 5\,\mathrm{K}$. To characterize the

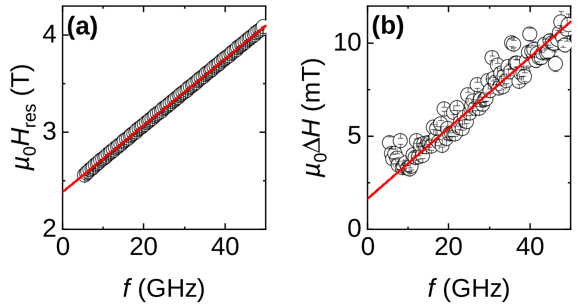


Figure S1. (a) Resonance field $\mu_0 H_{\mathrm{res}}(f)$ of the $Al_2O_3$/CoFe sample at $T = 5\,\mathrm{K}$ plotted versus frequency. The line shows a fit to Eq. (S1) and is used to extract $g$ and $M_{\mathrm{eff}}$. (b) Resonance linewidth $\mu_0 \Delta H(f)$ of the $Al_2O_3$/CoFe sample at $T = 5\,\mathrm{K}$ together with a fit to Eq. (S2) (red line) used to extract $H_{\mathrm{inh}}$ and $\alpha$.

effective magnetization $M_{\mathrm{eff}}$ and the $g$-factor of the magnetic system $g$, the frequency dependence of the resonance field $H_{\mathrm{res}}(f)$ is fitted using

$$\mu_0 H_{\mathrm{res}} = +\mu_0 M_{\mathrm{eff}} + \frac{h}{g\mu_{\mathrm{B}}} \cdot f, \tag{S1}$$

where $h$ is the Planck constant and $\mu_{\mathrm{B}}$ is the Bohr magneton. We extract a $g$-factor of $g = 2.079 \pm 0.001$ and an effective magnetization $\mu_0 M_{\mathrm{eff}} = (2.381 \pm 0.004)\,\mathrm{T}$ corresponding to the expected values for CoFe of this material composition ($Co_{25}Fe_{75}$)[1].

The frequency dependency of the FMR linewidth $\mu_0 \Delta H(f)$ is fitted with the linear model following Eq. (S2) to extract the Gilbert damping parameter $\alpha$, which is proportional to the slope of the $\mu_0 \Delta H(f)$-dependence and the

* manuel.mueller@wmi.badw.de
† matthias.althammer@wmi.badw.de
‡ hans.huebl@wmi.badw.de

inhomogeneous broadening $\mu_0 H_{\mathrm{inh}}$ as its $y$-axis intercept[1]

$$\mu_0 \Delta H(f) = \mu_0 H_{\mathrm{inh}} + 2 \cdot \frac{h\alpha}{g\mu_{\mathrm{B}}} \cdot f. \tag{S2}$$

We extract an inhomogeneous line broadening of $\mu_0 H_{\mathrm{inh}} = (1.6 \pm 0.2)\,\mathrm{mT}$ and a Gilbert damping $\alpha = (2.8 \pm 0.1) \cdot 10^{-3}$, which is in good agreement with the values reported in Ref. [1].

## II. Frequency splitting of the transverse acoustic phonon modes

In Fig. 3(b) of the main text and Fig. S2 we clearly can identify two resonant features of the BAW modes in our samples. Since we are in the linear regime of the phonon dispersion close to the center of the Brillouin zone, the resonance condition reads as $f_n = v_{\mathrm{t}}/\lambda_n$. Since $\lambda_n$ is fixed by the geometrical size of the BAW resonator, the observation of two different resonant frequencies provides clear evidence for the presence of different velocities of the two transverse acoustic phonon modes. That is, the velocities $v_{\mathrm{ft}}$ and $v_{\mathrm{st}}$ of the two transverse acoustic phonon modes are not degenerated but show a finite splitting. Here, we study this splitting around different $f_0$ ranging from 12 to 30 GHz for two CoFe samples grown on $\boldsymbol{c}$-axis oriented $Al_2O_3$ with different miscut specifications (see Fig. S2 and Tabs. SI and SII). We find that the observed frequency separation $\Delta f$ of the two standing phonon modes scales linearly with $f_0$. This is expected since (cf. Section IV)

$$\Delta f = f_n^{\mathrm{ft}} - f_n^{\mathrm{st}} = \frac{v_{\mathrm{ft}} - v_{\mathrm{st}}}{\lambda_n} \tag{S3}$$

and $\lambda_n$ decreases linearly with $f_0$.

For the second CoFe thin-film on a $Al_2O_3$ substrate with a miscut specification of $\theta_{\mathrm{m}} < 0.2°$, we find a larger slope of the $\Delta f(f_{\mathrm{FMR}})$ dependence corresponding to a larger difference $v_{\mathrm{ft}} - v_{\mathrm{st}}$ of the velocities of the two transverse acoustic phonon modes. The relation of $v_{\mathrm{ft}} - v_{\mathrm{st}}$ with the miscut angle of the substrate clearly suggests that $v_{\mathrm{ft}} - v_{\mathrm{st}}$ is related to the fact that the phonon propagation is no longer along $c$-axis and hence the velocities of the two phonon modes are no longer degenerate.

| $f_0$ (GHz) | 12 | 18 | 24 | 30 |
|---|---|---|---|---|
| $\mu_0 H_{\mathrm{res}}$ (T) | 2.80 | 3.01 | 3.21 | 3.42 |
| $\min(\lvert S_{21}\rvert)$ $(10^{-3})$ | 55 | 16 | 5.1 | 2.2 |
| $\max(\lvert S_{21}\rvert)$ $(10^{-3})$ | 75 | 26 | 8.6 | 4.0 |

Table SI. Plot parameters of Fig. 3(a). Frequency $f$, resonance field $\mu_0 H_{\mathrm{res}}$ as well as minimum and maximum $S_{21}$-parameter $\min(|S_{21}|)$ and $\max(|S_{21}|)$.

| $f_0$ (GHz) | 12 | 18 | 24 | 30 |
|---|---|---|---|---|
| $\mu_0 H_{\mathrm{res}}$ (T) | 2.78 | 3.00 | 3.21 | 3.41 |
| $\min(\lvert S_{21}\rvert)$ $(10^{-3})$ | 140 | 72 | 36 | 18 |
| $\max(\lvert S_{21}\rvert)$ $(10^{-3})$ | 156 | 86 | 46 | 24 |

Table SII. Plot parameters of Fig. 3(b). Frequency $f_0$ and corresponding resonance field $\mu_0 H_{\mathrm{res}}$ as well as minimum and maximum $S_{21}$-parameter $\min(|S_{21}|)$ and $\max(|S_{21}|)$.

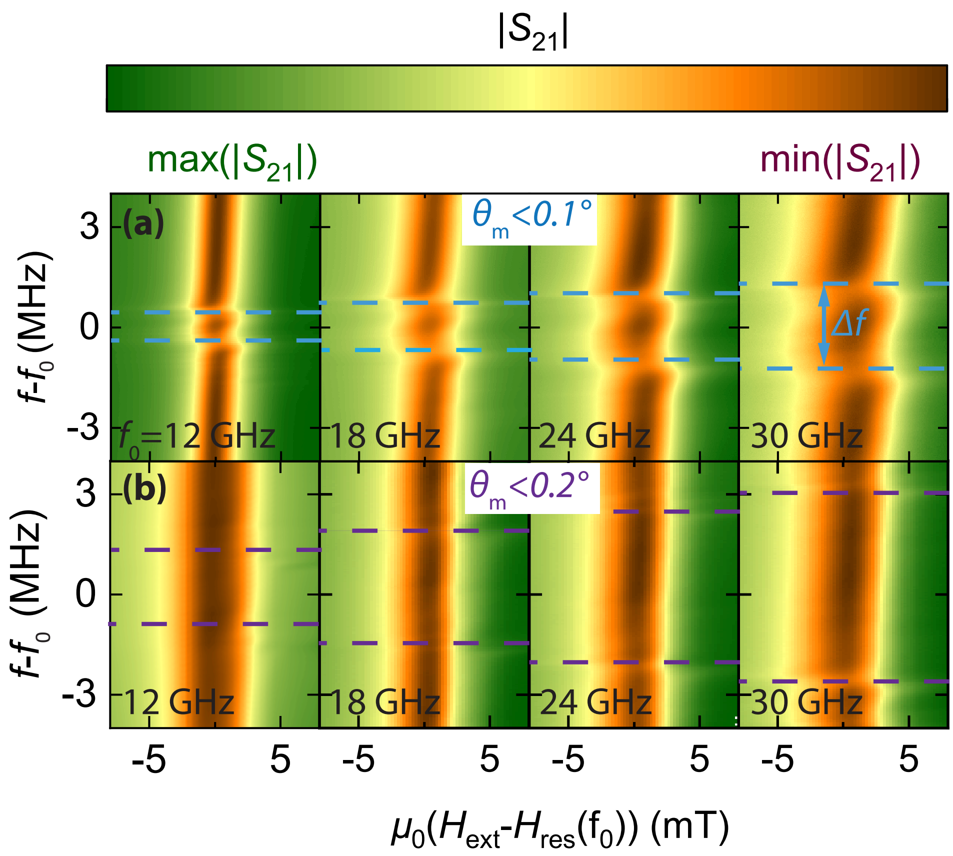


Figure S2. (a) Microwave transmission magnitude $|S_{21}|$ as a function of frequency $f$ and $H_{\rm ext}$ in narrow frequency regimes around different frequencies $f_0$ recorded at $T = 5\,$K for a CoFe thin film deposited on $c$-axis $Al_2O_3$ substrate with a miscut $\theta_{\rm m} < 0.1°$. Panel (b) shows a second sample of CoFe on a $c$-axis $Al_2O_3$ substrate with a specified miscut of $\theta_{\rm m} < 0.2°$ .The light blue and purple dashed lines are a guide to the eye indicating that $\Delta f$ scales linearly with $f_0$ for both samples. The $H_{\rm res}$ as well as min($|S_{21}|$) and max($|S_{21}|$) at the respective $f_0$ are given in Tabs. SI and SII. Note that the frequency spacing of the panels in (a) and (b) is 6 GHz.

## III. Theory model

To model the MEC coupling in Fig. 2(a), we use the formalism derived in Ref. [2]. In detail, we calculate the modified Polder susceptibility $\hat{\chi}_{\rm tot}$ in the presence of MEC coupling. In Fig. S3 we plot the experimentally observed $|S_{21}|$ in panel (a) together with the simulated spectrum of the absorbed power $P_{\rm abs}$ given by Eq.(36) in Ref.[2] in panel (b) as function of external field and frequency around $f_0 = 18\,$GHz. For our simulation, we use for the magnetization dynamics parameters the values extracted via broadband ferromagnetic resonance spectroscopy (BBFMR) in section I with $M_{\rm s} = M_{\rm eff} = 1.91083 \cdot 10^6\,$A/m, $\alpha = 2.8 \cdot 10^{-3}$, $\mu_0 H_{\rm inh} = 1.6\,$mT and $\gamma = g\mu_{\rm B}/\hbar = 29.13 \cdot 10^9 \cdot 2\pi\,1/$s. For the elastic properties of sapphire and CoFe (denoted with a tilde-accent), we use two transverse phonon velocities in sapphire $v_{\rm st} = 6170\,$m/s[3], $v_{\rm ft} = v_{\rm st} + \Delta v_{\rm t}$ with $\Delta v_{\rm t} = 0.5\,$m/s and for CoFe $\tilde{v}_{\rm t} = 3170\,$m/s[4]. Furthermore, we assume the mass densities $\rho_{\rm t} = 3970\,$kg/m$^3$ (Manufacturer specification) and $\tilde{\rho}_{\rm t} = 8110\,$kg/m$^3$[4]. For the elastic damping parameters of the two elastic waves in sapphire and CoFe, we use $\eta_{\rm a1}/(2\pi) = 0.23\,$MHz, $\eta_{\rm a2}/(2\pi) = 0.16\,$MHz determined from the data presented in the main text. Due to the low layer thickness of the CoFe layer, the elastic damping of the CoFe layer $\tilde{\eta}_{\rm a}$ can be neglected. Furthermore, we use the geometric properties $L = 510\,\mu$m and $d = 30\,$nm as well as $h_\parallel = h_\perp = 1$ for the parallel and perpendicular driving field components of the CPW. Finally, for the magnetoelastic constant $B$ in polycrystalline thin films, we use[5]

$$B = \frac{3}{2}\frac{E}{1+\nu}\lambda_{\rm s} \tag{S4}$$

where $E$ is the Young's modulus, $\nu$ is the Poisson ratio and $\lambda_{\rm s}$ is the saturation magnetostriction. We insert $E = 220\,$GPa[6], $v = 0.29$ (Sputtering target manufacturer's specification) and $\lambda_{\rm s} = 0.25\lambda_{\rm s}^{\rm Co} + 0.75\lambda_{\rm s}^{\rm Fe} \approx 6.1 \cdot 10^{-5}$[5] in

Eq. (S4) and obtain $B = 15.7 \cdot 10^6\ \mathrm{J/m^3}$.
Using these parameters, we observe in Fig. S3 a good agreement between the simulation and the experimental data. We observe a slight frequency shift between theory and experiments due to uncertainties in the thickness $L$ and

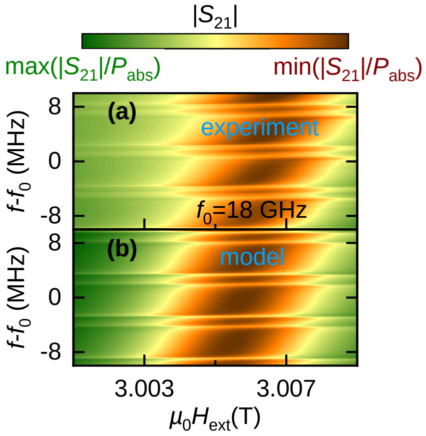


Figure S3. (a) $|S_{21}|$ recorded at $T = 5\,\mathrm{K}$ and plotted as a function of $f$ and $H_{\mathrm{ext}}$ in the range of $\mu_0 H_{\mathrm{res}} = 3.005\,\mathrm{T}$ corresponding to $f_0 = 18$ GHz. (b) Simulation of $P_{\mathrm{abs}}$ plotted as a function of $f$ and $H_{\mathrm{ext}}$ in the range of $H_{\mathrm{res}}$ for $f_0 = 18$ GHz using the parameters listed above. A good agreement between experiment and theory is observed. The plotted power absorption range is (a) from $\min(|S_{21}|) = 0.016$ to $\max(|S_{21}|) = 0.025$ and (b) from $\min(P_{\mathrm{abs}}) = 1.0 \cdot 10^{-4}$ to $\max(P_{\mathrm{abs}}) = 4.9 \cdot 10^{-4}$.

velocity $v_{\mathrm{t}}$ of the sapphire layer. From Fig. S3, we verify, that our assumed material parameters are valid. However, Ref. [2] does not provide an analytical expression of the effective magnetoelastic coupling strength $g_{\mathrm{eff}}(f)$.
Hence, to determine the coupling $g_{\mathrm{eff}}(f)$, we use [7, 8]

$$g_{\mathrm{eff}}(f)/(2\pi) = \frac{1}{2\pi} B \sqrt{\frac{2g\mu_{\mathrm{B}}}{hfM_{\mathrm{s}}\tilde{\rho}_{\mathrm{t}}dL}} \left[1 - \cos\left(2\pi f \frac{d}{\tilde{v}_t}\right)\right], \tag{S5}$$

Using $M_s = M_{\mathrm{eff}}$, $L = 510\,\mu\mathrm{m}$ and $d = 30\,\mathrm{nm}$, the transverse velocity $\tilde{v}_{\mathrm{st}} = 3170\,\mathrm{m/s}$ and $\tilde{\rho}_{\mathrm{t}} = 8110\,\mathrm{kg/m^3}$ for the volume density in CoFe[4] as well as $B = 15.7 \cdot 10^6\ \mathrm{J/m^3}$, we obtain $g_{\mathrm{eff}}(f_0)/(2\pi) \approx 6.0$ MHz at $f_0 = 18\,\mathrm{GHz}$.
To prove the validity of this approach, we apply the same formalism as in Ref. [7] and describe our systems as two uncoupled elastic wave modes, each individually coupled to the magnetic Kittel mode. The set of differential equations describing such a model is

$$\begin{aligned}
(f - f_{\mathrm{m}} + i\kappa_s/(2\pi))m^{\mathrm{x}} &= g_1 u_n^{\mathrm{x}}/(4\pi) + \zeta h^{\mathrm{x}} \\
(f - f_{\mathrm{m}} + i\kappa_s/(2\pi))m^{\mathrm{y}} &= g_2 u_n^{\mathrm{y}}/(4\pi) + \zeta h^{\mathrm{y}} \\
(f - f_{\mathrm{n}}^{\mathrm{x}} + i\eta_{\mathrm{a1}}/(2\pi))u_n^{\mathrm{x}} &= g_1 m^{\mathrm{x}}/(4\pi) \\
(f - f_{\mathrm{n}}^{\mathrm{y}} + i\eta_{\mathrm{a2}}/(2\pi))u_n^{\mathrm{y}} &= g_2 m^{\mathrm{y}}/(4\pi)
\end{aligned} \tag{S6}$$

Here, $f_{\mathrm{m}}$ is the magnetic resonance frequency determined by solving Eq. (S1) for $f$ and the $f_{\mathrm{n}1,2}$ are the resonance frequencies of the elastic standing waves using Eq. (1) of the main text with $v_{\mathrm{ft}}$ and $v_{\mathrm{st}}$. The variables $m^{\mathrm{x}}$ and $m^{\mathrm{y}}$ are the two linearly polarized magnetization amplitudes and likewise the $u_{\mathrm{n}}^{\mathrm{x}}$ and $u_{\mathrm{n}}^{\mathrm{y}}$ are the linearly polarized elastic wave amplitudes propagating at slightly different propagation velocities and hence being in resonance at the frequencies $f_{\mathrm{n}}^{\mathrm{x}}$ and $f_{\mathrm{n}}^{\mathrm{y}}$.Note, that we can assume that $m_{\mathrm{x}}$ is coupled exclusively to $f_{\mathrm{x}}$ and $m_{\mathrm{y}}$ solely to $f_{\mathrm{y}}$, as we are free to define the x-y-coordinate system of the FMR with respect to the polarization of the acoustic modes. The parameter $\zeta$ describes the inductive coupling to the antenna and $h^{\mathrm{x}}$ and $h^{\mathrm{y}}$ are the driving field of the coplanar waveguide. The power absorption of this system is given by $P_{\mathrm{abs}} = \zeta(h^{\mathrm{x}}\mathrm{Im}(m^{x}) + h^{\mathrm{y}}\mathrm{Im}(m^{y}))$. In Fig. S4, we plot $P_{\mathrm{abs}}$ using the elastic and magnetic loss rates $\eta_{\mathrm{a1}}/(2\pi) = 0.23\,\mathrm{MHz}$, $\eta_{\mathrm{a2}}/(2\pi) = 0.16\,\mathrm{MHz}$, $\kappa_s/(2\pi) = 69.0\,\mathrm{MHz}$ as for Fig. S3 from the main text, an effective coupling strength of $g_1/(2\pi) = g_2/(2\pi) = 6.0\,\mathrm{MHz}$, $\zeta = 1\,\mathrm{MHz}$ and $h^{\mathrm{x}} = h^{\mathrm{y}} = 1$. We again observe in Fig. S4 a good agreement between theory model and the experimental data, demonstrating, that the magnitude of our assumed coupling is in agreement with theoretical predictions.

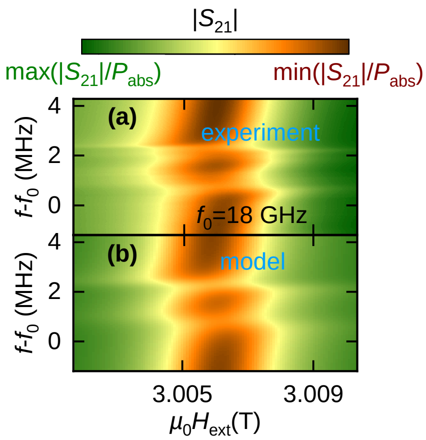


Figure S4. (a) $|S_{21}|$ recorded at $T = 5\,\mathrm{K}$ and plotted as a function of $f$ and $H_{\mathrm{ext}}$ in the range of $H_{\mathrm{res}}$ for $f_0 = 18$ GHz corresponding to the $n = 2918^{\mathrm{th}}$ BAW resonance mode number ($f_0 \approx f_{2918}^{\mathrm{x/y}}$). (b) Simulation of $P_{\mathrm{abs}}$ obtained by solving Eq. (S6) by $m^{\mathrm{x}} + m^{\mathrm{y}}$ and plotted as a function of $f$ and $H_{\mathrm{ext}}$ in the range of $H_{\mathrm{res}}$ for $f_0 = 18$ GHz using the parameters listed above. A good agreement between experiment and theory is observed. The plotted power absorption range is (a) from $\min(|S_{21}|) = 0.016$ to $\max(|S_{21}|) = 0.025$ and (b) from $\min(P_{\mathrm{abs}}) = 0.24 \cdot 10^6$ to $\max(P_{\mathrm{abs}}) = 2.52 \cdot 10^6$.

## IV. Analytical expression for the frequency-splitting of the acoustic resonances for the two transverse modes $\Delta f(f)$

The acoustic resonance condition of slow/fast transverse phonons is given by [2]

$$f_n^{\mathrm{ft/st}} = \frac{n}{2(d/\tilde{v}_t + L/v_{\mathrm{ft/st}})}. \tag{S7}$$

Hence the expected frequency splitting between these acoustic resonances $\Delta f$ for the same mode number $n$ is given by:

$$\begin{aligned}\Delta f_n &= f_n^{\mathrm{ft}} - f_n^{\mathrm{st}} = \frac{n}{2(d/\tilde{v}_{\mathrm{t}} + L/v_{\mathrm{ft}})} - \frac{n}{2(d/\tilde{v}_{\mathrm{t}} + L/v_{\mathrm{st}})} = \\ &= \frac{1}{2f_{\mathrm{FSR}}} \frac{L\tilde{v}_{\mathrm{t}}^2(v_{\mathrm{ft}} - v_{\mathrm{st}})}{(dv_{\mathrm{ft}} + L\tilde{v}_t)(dv_{\mathrm{st}} + L\tilde{v}_t)} \cdot f \approx \frac{1}{2f_{\mathrm{FSR}}L}\Delta v_{\mathrm{t}} \cdot f = \\ &= a \cdot f\end{aligned} \tag{S8}$$

Here, we used $n = f/f_{\mathrm{FSR}}$ and $\Delta v_{\mathrm{t}} = v_{\mathrm{ft}} - v_{\mathrm{st}}$. The approximation made in Eq. (S8) is valid for $dv_{\mathrm{ft/st}} \ll L\tilde{v}_{\mathrm{t}}$, which is the case in our experiments. We find a linear relation between $\Delta f$ and $f$ with a slope $a$ that is proportional to the difference of the transverse velocities $\Delta v_{\mathrm{t}}$.

## V. Frequency splitting $\Delta f(f)$ of the transverse modes for the substrate materials investigated in this study.

The frequency splitting $\Delta f(f)$ of the MEC double peak features recorded at $T = 5\,\mathrm{K}$ as function of $f$ around $f_0 = 18\,\mathrm{GHz}$ for CoFe deposited on various substrate materials is shown for all of the investigated substrate materials in Fig. S5. The observed behavior in $\Delta f(f)$ can be well fitted with a linear function without a zero y-axis intercept following Eq. (S8). As a general trend, the slope $a$ of the fits in Fig. S5 is larger for substrate materials with a larger potential miscut angle $\theta_{\mathrm{m}}$ and larger $v_{\mathrm{t}}$.

## VI. Theory model for the velocity splitting of the transverse modes

In the main text, we have used the Christoffel Python tool from Ref. [9] to calculate the dispersion of the transverse modes and thus $v_{\mathrm{ft}}$ and $v_{\mathrm{st}}$ as function of the phonon propagation direction. Here, we derive the exact analytical expression for the transverse velocity splitting as function of the relative propagation direction with respect to a

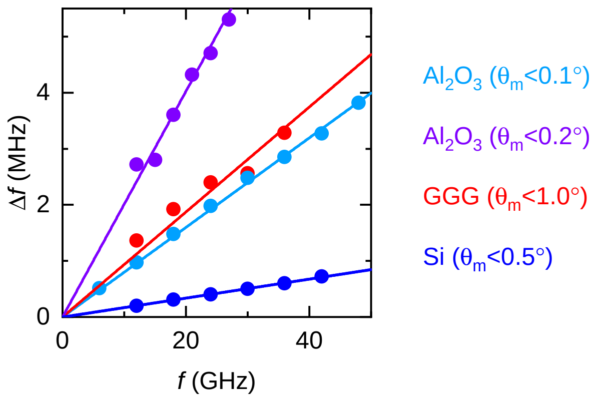


Figure S5. Frequency splitting $\Delta f(f)$ of the MEC double peak features recorded at $T = 5\,\mathrm{K}$ as function of $f$ around $f_0$ =18 GHz for CoFe deposited on various substrate materials. A linear evolution as function of $f$ following Eq. (S8) is confirmed for all substrate materials studied in this work.

selected crystallographic axis given by the angle $\theta$.

### VI.I. Substrate with hexagonal crrystallographic order

We start by deriving the dispersion relation and the acoustic phonons and their respective group velocities of the sapphire layer taking into account the relative directions between the $c$-axis and the phonon propagation. The components of the stress tensor of the sapphire layer can be written as [10]

$$\begin{aligned}
\sigma_{x,x} &= c_{11}\varepsilon_{x,x} + c_{12}\varepsilon_{y,y} + 2c_{14}\varepsilon_{y,z} + c_{13}\varepsilon_{z,z} \\
\sigma_{y,y} &= c_{12}\varepsilon_{x,x} + c_{11}\varepsilon_{y,y} - 2c_{14}\varepsilon_{y,z} + c_{13}\varepsilon_{z,z} \\
\sigma_{z,z} &= c_{13}\varepsilon_{x,x} + c_{13}\varepsilon_{y,y} + c_{33}\varepsilon_{z,z} \\
\sigma_{y,z} &= \sigma_{z,y} = c_{14}\varepsilon_{x,x} - c_{14}\varepsilon_{y,y} + 2c_{44}\varepsilon_{y,z} \\
\sigma_{x,z} &= \sigma_{z,x} = 2c_{14}\varepsilon_{x,y} + 2c_{44}\varepsilon_{x,z} \\
\sigma_{x,y} &= \sigma_{y,x} = (c_{11} - c_{12})\,\varepsilon_{x,y} + 2c_{14}\varepsilon_{x,z}
\end{aligned} \tag{S9}$$

where $c_{pq}$ represents the components of the stiffness tensor in Voigt notation, and $\varepsilon_{i,j}$ is the strain tensor. We reshape the strain tensor taking into account the deflection of $c$-axis by introducing an auxiliary cartesian coordinate system $\{x', y', z'\}$. The transformation of the strain tensor into the $x'y'z'$-system is given by

$$\varepsilon_{i',j'} = \sum_{k,j} \left(R^T\right)_{i',j} \varepsilon_{j,k} R_{k,j'} \,,$$

where the Euler matrix reads

$$R = \begin{pmatrix} \cos\theta & 0 & \sin\theta \\ 0 & 1 & 0 \\ -\sin\theta & 0 & \cos\theta \end{pmatrix} .$$

This matrix describes the rotation of the $c$-axis by a $\theta$ angle. In the following we omit prime superscripts in the notation, since we do not have $\varepsilon_{i,j}$ in the following equations. Based on the written expressions, we reshape the stress tensor in terms of displacement $u$ using

$$\varepsilon_{i,j} = \frac{1}{2}\left(\frac{\partial u_i}{\partial x_j} + \frac{\partial u_j}{\partial x_i}\right) ,$$

where coordinates are denoted as $\{x_x, x_y, x_z\}$. If we write the force density in the form

$$f_i = \sum_j \frac{\partial \sigma_{i,j}}{\partial x_j}\,,$$

then Hooke's equation of motion reads

$$\rho \frac{\partial^2 \mathbf{u}}{\partial t^2} + \delta \frac{\partial \mathbf{u}}{\partial t} = \mathbf{f}\,, \tag{S10}$$

where $\rho$ is the mass density, and $\delta = \eta_{\rm a}\rho$. The components of the above equation read (for $\theta = 0°$)

$$\begin{aligned}
\rho \frac{\partial^2 u_x}{\partial t^2} &= -\eta \frac{\partial u_x}{\partial t} + \frac{1}{2}c_{11}\left(u_x^{(0,2,0)} + u_y^{(1,1,0)} + 2u_x^{(2,0,0)}\right) + \frac{1}{2}c_{12}\left(u_y^{(1,1,0)} - u_x^{(0,2,0)}\right) \\
&\quad + c_{13}u_z^{(1,0,1)} + c_{44}\left(u_x^{(0,0,2)} + u_z^{(1,0,1)}\right) + 2c_{14}\left(u_x^{(0,1,1)} + u_y^{(1,0,1)} + u_z^{(1,1,0)}\right), \\
\rho \frac{\partial^2 u_y}{\partial t^2} &= -\eta \frac{\partial u_y}{\partial t} + \frac{1}{2}c_{11}\left(2u_y^{(0,2,0)} + u_x^{(1,1,0)} + u_y^{(2,0,0)}\right) + \frac{1}{2}c_{12}\left(u_x^{(1,1,0)} - u_y^{(2,0,0)}\right) \\
&\quad + c_{13}u_z^{(0,1,1)} + c_{44}\left(u_y^{(0,0,2)} + u_z^{(0,1,1)}\right) - c_{14}\left(2u_y^{(0,1,1)} + u_z^{(0,2,0)} - 2u_x^{(1,0,1)} - u_z^{(2,0,0)}\right), \\
\rho \frac{\partial^2 u_z}{\partial t^2} &= -\eta \frac{\partial u_z}{\partial t} + c_{13}\left(u_y^{(0,1,1)} + u_x^{(1,0,1)}\right) + c_{14}\left(-u_y^{(0,2,0)} + 2u_x^{(1,1,0)} + u_y^{(2,0,0)}\right) \\
&\quad + c_{33}u_z^{(0,0,2)} + c_{44}\left(u_y^{(0,1,1)} + u_z^{(0,2,0)} + u_x^{(1,0,1)} + u_z^{(2,0,0)}\right).
\end{aligned}$$

The spatial derivatives are denoted with superscripts, i.e. ${u_z}^{(1,1,0)} = \dfrac{\partial^2 u_z}{\partial x \partial y}$, ${u_z}^{(0,0,2)} = \dfrac{\partial^2 u_z}{\partial z^2}$, and etc. We use the plane wave ansatz

$$u_{x,y,z} = u_{x,y,z} e^{i(\omega t - \mathbf{k}\cdot\mathbf{r})}.$$

Next, we focus on standing waves along the thickness of the sapphire, hence the wave vector has only one component $k = k_z = n\pi/L$. Thus, the Hooke's equation yields a dispersion equation, which can be written in matrix form

$$\det \begin{pmatrix} a_{11} & a_{12} & a_{13} \\ a_{21} & a_{22} & a_{23} \\ a_{31} & a_{32} & a_{33} \end{pmatrix} = 0, \tag{S11}$$

where

$$\begin{aligned}
a_{11} &= c_{44}k^2\cos(2\theta) + i\omega\eta - \rho\omega^2\,, \\
a_{12} &= -c_{14}k^2\sin(\theta)\,, \\
a_{13} &= -c_{44}k^2\sin(2\theta)\,, \\
a_{21} &= -c_{14}k^2\sin(\theta)\cos(\theta)\,, \\
a_{22} &= c_{44}k^2\cos(\theta) + i\eta\omega - \rho\omega^2\,, \\
a_{23} &= c_{14}k^2\sin^2(\theta)\,, \\
a_{31} &= (c_{13} - c_{33})\,k^2\sin(\theta)\cos(\theta)\,, \\
a_{32} &= 0\,, \\
a_{33} &= -k^2\left(c_{13}\sin^2(\theta) + c_{33}\cos^2(\theta)\right) + \rho\omega^2 - i\eta\omega\,.
\end{aligned} \tag{S12}$$

The group velocities of the acoustic waves can be calculated as

$$v_g = \frac{\partial \omega}{\partial k}\,.$$

The explicit form of this equation is not elucidating, we therefore turn to numerical results for the exact solution. We find that the velocities of two acoustic waves are almost the same $v_g \approx 6.17$ km/s for the parameters listed in Fig. S6, the difference between them depends on the deflection angle $\theta$ away from the $c$-axis as shown in Fig. S6. For a miscut angle of $\theta = 0.017°$, we obtain $\Delta v \approx 0.5\,\text{m/s}$ in agreement with the calculations in the main text using the simplified Christoffel equation[9].

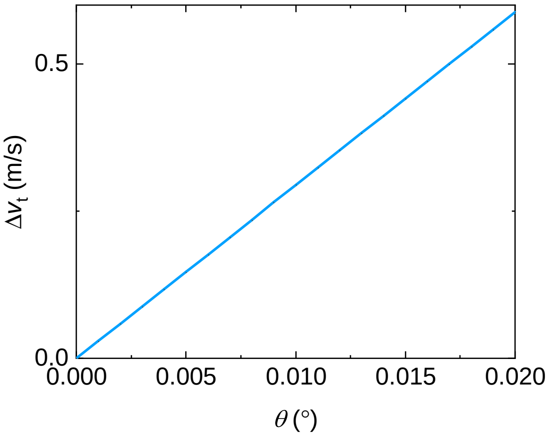


Figure S6. The difference between velocities of two acoustic waves measured in hexagonal $Al_2O_3$. The calculation parameters are $k = 2\pi/L$ rad $\cdot$ m$^{-1}$, $L = 510$ $\mu$m, $\rho = 3970$ kg/m$^3$, $c_{11} = 5.00073 \times 10^{11}$ Pa, $c_{33} = 5.02385 \times 10^{11}$ Pa, $c_{44} = 1.51017 \times 10^{11}$ Pa, $c_{12} = 1.61672 \times 10^{11}$ Pa, $c_{13} = 1.11368 \times 10^{11}$ Pa, $c_{14} = -2.32604 \times 10^{10}$ Pa and $\eta_a/(2\pi) = 0.23$ MHz. These tensor elements are extracted from Ref. [3].

## VI.II. Cubic crystallographic order

We employ the same formalism to derive the velocity difference $\Delta v$ of acoustic waves in an elastic medium with cubic symmetry. In a cubic system, the stress tensor elements are given by[10]

$$
\begin{aligned}
\sigma_{x,x} &= c_{11}\varepsilon_{x,x} + c_{12}\varepsilon_{y,y} + c_{12}\varepsilon_{z,z} , \\
\sigma_{y,y} &= c_{12}\varepsilon_{x,x} + c_{11}\varepsilon_{y,y} + c_{12}\varepsilon_{z,z} , \\
\sigma_{z,z} &= c_{12}\varepsilon_{x,x} + c_{12}\varepsilon_{y,y} + c_{11}\varepsilon_{z,z} , \\
\sigma_{y,z} &= \sigma_{z,y} = 2c_{44}\varepsilon_{y,z} , \\
\sigma_{x,z} &= \sigma_{z,x} = 2c_{44}\varepsilon_{x,z} , \\
\sigma_{x,y} &= \sigma_{y,x} = 2c_{44}\varepsilon_{x,y} .
\end{aligned}
$$

Performing the same procedure as before, the dispersion equation is given by

$$
\det \begin{pmatrix} c_{44}k^2\cos(2\theta) - \rho\omega^2 + i\delta\omega & 0 & -2c_{44}k^2\sin(\theta)\cos(\theta) \\ 0 & c_{44}k^2\cos(\theta) - \rho\omega^2 + i\delta\omega & 0 \\ (c_{11} - c_{12})\, k^2\sin(\theta)\cos(\theta) & 0 & c_{12}k^2\sin^2(\theta) + c_{11}k^2\cos^2(\theta) - \rho\omega^2 + i\delta\omega \end{pmatrix} = 0.
$$

The calculated $\Delta v$ solving this equation is plotted in Fig. S7.

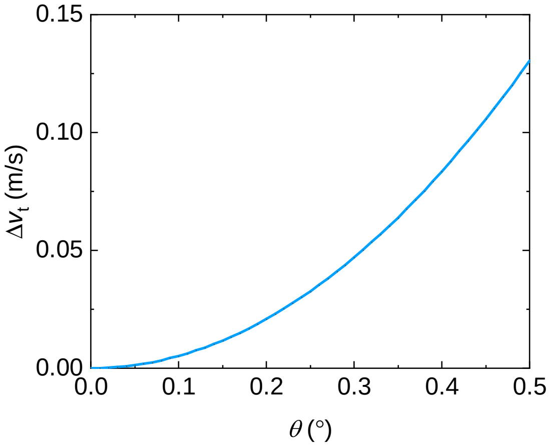


Figure S7. The difference between velocities of two acoustic waves measured in cubic Si. The calculation parameters are $k = 2\pi/L$ rad $\cdot$ m$^{-1}$, $L = 510$ $\mu$m, $\rho = 3970$ kg/m$^3$, $c_{11} = 161.8$ GPa, $c_{12} = 64$ GPa, $c_{44} = 76.1$ $G$Pa and $\eta_a/(2\pi) = 0.23$ MHz. These tensor elements are extracted from Ref. [11].


[1] L. Flacke, L. Liensberger, M. Althammer, H. Huebl, S. Geprägs, K. Schultheiss, A. Buzdakov, T. Hula, H. Schultheiss, E. R. J. Edwards, H. T. Nembach, J. M. Shaw, R. Gross, and M. Weiler, High spin-wave propagation length consistent with low damping in a metallic ferromagnet, Appl. Phys. Lett. **115**, 122402 (2019).

[2] T. Sato, W. Yu, S. Streib, and G. E. W. Bauer, Dynamic magnetoelastic boundary conditions and the pumping of phonons, Phys. Rev. B **104**, 014403 (2021).

[3] W. E. Tefft, Elastic constants of synthetic single crystal corundum, J. Res. Natl. Bur. Stand. A (U. S.) **70A**, 277 (1966).

[4] D. Schwienbacher, M. Pernpeintner, L. Liensberger, E. R. J. Edwards, H. T. Nembach, J. M. Shaw, M. Weiler, R. Gross, and H. Huebl, Magnetoelasticity of $Co_{25}Fe_{75}$ thin films, Journ. Appl. Phys. **126**, 103902 (2019).

[5] E. Klokholm and J. Aboaf, The saturation magnetostriction of thin polycrystalline films of iron, cobalt, and nickel, Journ. Appl. Phys. **53**, 2661 (1982).

[6] M. Yamamoto, Young's Modulus of Elasticity and Its Change with Magnetization in Iron-Cobalt Alloys, Phys. Rev. **59**, 768 (1941).

[7] K. An, A. N. Litvinenko, R. Kohno, A. A. Fuad, V. V. Naletov, L. Vila, U. Ebels, G. De Loubens, H. Hurdequint, N. Beaulieu, J. Ben Youssef, N. Vukadinovic, G. E. Bauer, A. N. Slavin, V. S. Tiberkevich, and O. Klein, Coherent long-range transfer of angular momentum between magnon Kittel modes by phonons, Phys. Rev. B **101**, 1 (2020).

[8] R. Schlitz, L. Siegl, T. Sato, W. Yu, G. E. W. Bauer, H. Huebl, and S. T. B. Goennenwein, Magnetization dynamics affected by phonon pumping, Phys. Rev. B **106**, 014407 (2022).

[9] J. W. Jaeken and S. Cottenier, Solving the Christoffel equation: Phase and group velocities, Comput. Phys. Commun. **207**, 445 (2016).

[10] J. F. Nye et al., Physical properties of crystals (Oxford university press, 1985).

[11] C. Malica and A. D. Corso, Quasi-harmonic temperature dependent elastic constants: applications to silicon, aluminum, and silver, J. Phys. Condens. Matter. **32**, 315902 (2020).
